# Supplementary material for: Electric dipole spin resonance at shallow donors in quantum wires
Source: arXiv:1812.08048 source file (2019-01-31)
Supplement: Supplementary file 1 [file Supplement_02_12_2018.pdf]

# Supplemental Material for " Electric dipole spin resonance for shallow donors in quantum wires"

D.V. Khomitsky,[1] E.A. Lavrukhina,[1] and E.Ya. Sherman[2,3]

[1] *Department of Physics, National Research Lobachevsky State University of Nizhni Novgorod, 603950 Gagarin Avenue 23, Nizhny Novgorod, Russian Federation*

[2] *Department of Physical Chemistry, The University of the Basque Country, 48080 Bilbao, Spain*

[3] *IKERBASQUE Basque Foundation for Science, Bilbao, Spain*

(Dated: December 2, 2018)

We consider dynamics of a multi-level system described by a non-stationary Schrödinger equation

$$i\hbar\frac{\partial\Psi(x,t)}{\partial t} = H\Psi(x,t), \tag{1}$$

where the total Hamiltonian $H = H_0 + V(t)$ is the sum of a stationary part $H_0$ and a time-periodic term $V(t+T) = V(t)$. Here $T$ is the period of the external field and, thus $H(t+T) = H(t)$. Although the full numerical solution of Eq. (1) for an arbitrary time $t$ is numerically demanding, the wavefunction at $t = NT$ where $N$ is an integer, can be obtained with a moderate computational effort since the entire information about this "stroboscopic" evolution can be extracted from the behavior of the system at $0 < t < T$.

For the periodic driving we apply the Floquet technique [1] for evolution of quantum systems to access this stroboscopic behavior [2–5] where the state at $t = NT$ is obtained from the initial one by the $N$-th power of a unitary single-period propagator. For this purpose, we first represent a state $\Psi(x,t)$ as a superposition over the basis $\psi_l(x)$, $(l = 1,\ldots,l_{\max})$ of the eigenstates of $H_0$ satisfying condition $H_0\psi_l(x) = E_l\psi_l(x)$. This superposition has the form:

$$\Psi(x,t) = \boldsymbol{C}^{\mathrm{T}}(t)\boldsymbol{\psi}(x), \tag{2}$$

where $\boldsymbol{C}(t)$ is the vector with $l_{\max}$ components, $\boldsymbol{\psi}(x) = \left(\psi_1(x),\ldots,\psi_{l_{\max}}(x)\right)^{\mathrm{T}}$, and it is convenient to write for the components of $\boldsymbol{C}(t)$: $C_l(t) \equiv c_l(t)e^{-iE_lt/\hbar}$. After substituting (2) into Eq. (1) we obtain a system of ordinary differential equations for the time-dependent coefficients $c_l(t)$. After its numerical solution on a single period of the driving potential, the single-period propagator $\mathbf{U}_{ln}(T)$ is constructed by the approach proposed in Ref. [2, 3] as follows. We perform an accurate calculation of the evolution for a specially chosen initial state $c_n(0) = \delta_{n,n_0}$ with a given $n_0$ on a single period of the driving field, where $n_0$ runs over all the basis states of the model. For each initial $n_0$ the resulting vector $\boldsymbol{C}(T)$ forms the $n_0$-th column of the single period propagator matrix $\mathbf{U}_{ln}(T)$. After this matrix is formed, we perform its numerical diagonalization and obtain the eigenvalues $E_Q$ which are the quasienergies of the driven system, and the corresponding orthogonal normalized eigenvectors with the components $A_l^Q$. The matrix $\mathbf{U}_{ln}(T)$ can thus be represented in the following form [2]:

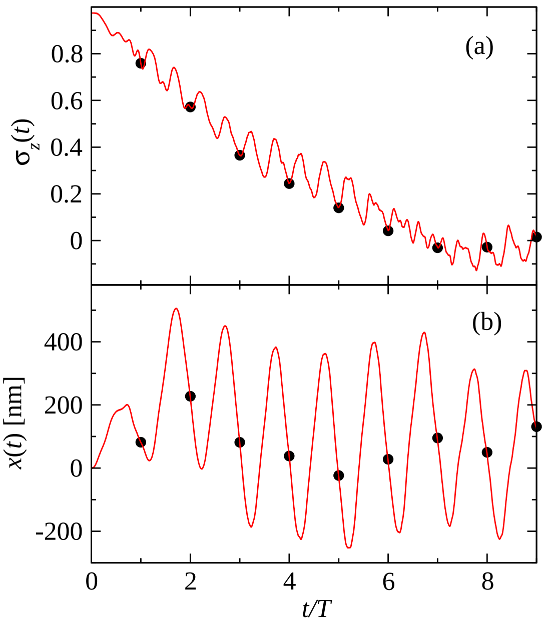


FIG. S1: Comparison of stroboscopic (black circles) and exact (solid lines) time dependences. The parameters correspond to Fig. 2 of the main text with $B = 0.5B_{\mathrm{m}}$, $F_0 = 1.5$ V/cm, and $\alpha = 6$ meVnm.

$$\mathbf{U}_{ln}(T) = \sum_Q A_l^Q \left(A_n^Q\right)^* e^{-iE_QT/\hbar}. \tag{3}$$

Its $N$-th power obtained by taking into account this orthogonality and normalization gives the stroboscopic propagator $\mathbf{U}_{ln}(NT)$ for $N$ periods as

$$\mathbf{U}_{ln}(NT) = \sum_Q A_l^Q \left(A_n^Q\right)^* e^{-iE_QNT/\hbar}, \tag{4}$$

and $\boldsymbol{C}(NT) = \mathbf{U}_{ln}(NT)\boldsymbol{C}(0)$.

The similarity of Eq. (3) for a single-period propagator and Eq. (4) for any $N \geq 1$ is a highly nontrivial fact demonstrating that $\mathbf{U}_{ln}(NT) = \mathbf{U}_{ln}^N(T)$. The stroboscopic approach allows us to study very accurately the long-time evolution since the $N$-period propagator (4) is constructed explicitly in a finite algebraic form. If we are interested in slowly evolving phenomena such as Rabi spin oscillations which occur here on many periods of the

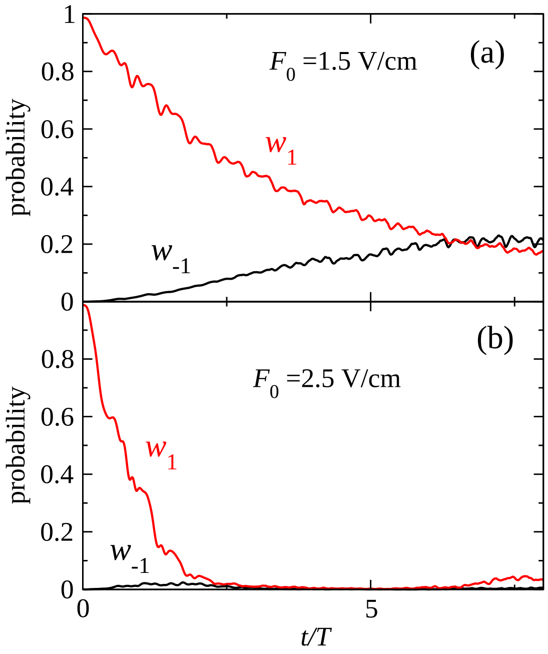


FIG. S2: Probabilities $w_1$ and $w_{-1}$ as functions of time for $B = 0.5B_\mathrm{m}$ and $\alpha = 6$ meVnm: (a) $F_0 = 1.5$ V/cm and (b) $F_0 = 2.5$ V/cm.

driving field, the stroboscopic approach is fully justified and highly efficient. An example for the system of interest as described in the main text is given in Fig. S1. Note that although the driving is periodic, the irregular spectrum of the quasienergies makes the stroboscopic evolution highly aperiodic on the observation time scale.

One can see that the dynamics of $\sigma_z(t)$ in Fig. S1(a) is accurately described by the stroboscopic points which are accompanied only by low deviation oscillations. The fast position dynamics $x(t)$ in Fig. S1(b) is also described with a high precision. For this quantity the exact numerical approach naturally gives oscillations with the amplitude higher than that given by the stroboscopic picture. This difference in the behavior of spin and position is due to the stronger coupling of the electron position to the driving electric field than that for the spin, which evolution is mediated by the spin-orbit coupling. However, the overall pattern of the coordinate dynamics can be tracked either from continuous or stroboscopic picture with comparable outcome, which makes the stroboscopic approach valuable for studying various observables.

To study the details of the short-time dynamics, we introduce probabilities to find electron in the states $\psi_0^{\lambda=-1}$ and $\psi_0^{\lambda=1}$ defined by Eq. (6) in main text as

$$w_{-1} = |\langle\psi_0^{\lambda=-1}|\Psi(x,t)\rangle|^2, \qquad w_1 = |\langle\psi_0^{\lambda=1}|\Psi(x,t)\rangle|^2, \tag{5}$$

and plot them in Fig. S2 for two different driving fields. These results, which should be compared with Fig. 3(a) in the main text, show that the spin evolution and the decrease in the total probability $w_1 + w_{-1}$, occur on the timescales of the same order of magnitude, confirming the direct involvement of the continuum in the spin dynamics. Note that the initial spin-up population decreases at $5\ldots10$ periods of the driving field, i.e. on the time scale of a nanosecond. These numbers indicate promising conditions for spin manipulation in our system.


[1] J. H. Shirley, Phys. Rev. **138**, B979 (1965).
[2] L.E. Reichl, *The Transition to Chaos. Conservative Classical Systems and Quantum Manifestations*, 2nd Ed., Springer-Verlag, New York, 2004.
[3] V. Ya. Demikhovskii, F. M. Izrailev, and A. I. Malyshev, Phys. Rev. E **66**, 036211 (2002); Phys. Rev. Lett. **88**, 154101 (2002).
[4] D.V. Khomitsky, L.V. Gulyaev, and E.Ya. Sherman, Phys. Rev. B **85**, 125312 (2012).
[5] D.V. Khomitsky, A.I. Malyshev, E.Ya. Sherman, and M. Di Ventra, Phys. Rev. B **88**, 195407 (2013).
